# Supplementary material for: The chromium dimer: closing a chapter of quantum chemistry
Source: arXiv:2206.10738 ancillary file (2022-08-24)
Supplement: Supplementary file 1 [file supplemental.pdf]

# Supplementary information for
# "The chromium dimer: closing a chapter of quantum chemistry"

Henrik R. Larsson,[1,2] Huanchen Zhai,[1] C. J. Umrigar,[3] and Garnet Kin-Lic Chan[1,a)]
[1)] *Division of Chemistry and Chemical Engineering, California Institute of Technology, Pasadena, CA 91125, USA*
[2)] *Department of Chemistry and Biochemistry, University of California, Merced, CA 95343, USA*[b)]
[3)] *Laboratory of Atomic and Solid State Physics, Cornell University, Ithaca, NY 14853, USA*

## S1. ELECTRONIC STRUCTURE

Our simulations for the electronic structure of the $X^1\Sigma_g^+$ $Cr_2$ ground state were based on the composite method presented in the main text. It consists of an estimate of the exact binding energy at the cc-pVDZ-DK basis set level[1] (correlating 28 electrons in 76 orbitals), corrected for the basis-set limit (CBS) by the second order matrix-product-state-approximated multireference retaining the excitation degree perturbation,[2–5] MPS-REPT2, level of theory. All computations were based on the spin-free exact-two-component Hamiltonian,[6,7] and used PySCF,[8,9] BLOCK2,[5,10] and ARROW.[11–13] The composite binding energies, $\Delta E(R) = E(R) - E(\infty)$, at each interatomic distance $R$, were calculated by

$$\Delta E = \Delta E_{\mathrm{PDZ}}(\text{“exact”}) + \Delta E_{\mathrm{CBS}}(\text{MPS-REPT2}) - \Delta E_{\mathrm{DZ}}(\text{MPS-REPT2}), \tag{S1}$$

where we have omitted the $R$-dependence, for simplicity. To compare with experiment, following Li et al.,[12] we subtracted a zero-point energy of 0.029 eV from the experimental PEC.

### A. PDZ energies

The estimates of the exact energies at the cc-pVDZ-DK basis set level were computed as the average of energies from two distinct methods. The first method is selected heat bath configuration interaction plus perturbation theory (SHCI), which we took directly from Ref. 12. Using extrapolation this provides an estimate of the exact energy in the basis; the used data is shown in Table S1. For calculating the binding energies, the energy of the Cr atom was taken from the SHCI calculations with a value of $-1049.93257\,\mathrm{E_H}$, which is in very good agreement with a previous DMRG estimate of $-1049.93254\,\mathrm{E_H}$.[14] For the most difficult case, the optimization at $R = 2.25$ Å, the variational part of the SHCI computation took about 60 hours on 2 nodes each with 80 Intel Xeon E7-8880 CPUs. Computing the perturbative correction took 15 hours using one node of the same configuration.

TABLE S1. SHCI energies in $\mathrm{E_H}$ at the cc-pVDZ-DK level. Shown are the best variational, perturbative, and extrapolated energies in $\mathrm{E_H}$. The energies are shifted by $2099\,\mathrm{E_H}$.

| $R$/Å | $E$(var) | $E$(pt) | $E$(extrap.) |
|---|---|---|---|
| 1.50 | −0.8761 | −0.8901 | −0.8928 |
| 1.55 | −0.8907 | −0.9053 | −0.9084 |
| 1.60 | −0.8984 | −0.9137 | −0.9173 |
| 1.68 | −0.9019 | −0.9185 | −0.9229 |
| 1.80 | −0.8981 | −0.9165 | −0.9221 |
| 2.00 | −0.8889 | −0.9101 | −0.9178 |
| 2.25 | −0.8827 | −0.9046 | −0.9126 |
| 2.50 | −0.8813 | −0.9020 | −0.9096 |
| 2.75 | −0.8775 | −0.8973 | −0.9049 |
| 3.00 | −0.8722 | −0.8909 | −0.8984 |
| 3.25 | −0.8658 | −0.8840 | −0.8908 |

The second method is spin-adapted DMRG, computed using BLOCK2.[10] We used natural orbitals obtained by diagonalizing the spin-summed unrestricted coupled cluster singles and doubles (UCCSD) density matrix. We optimized the orbital ordering with a genetic algorithm[15] at $R = 2$ Å. The accuracy of the DMRG is controlled by a single parameter, the bond dimension $D$. The DMRG optimizations used a maximum bond dimension between $D_{\max} = 18,000$ and $28,000$, depending on the convergence at each bond distance. One DMRG iteration (sweep) at $D_{\max} = 28,000$ took around 20 hours on five nodes with 24-core Intel Xeon 8276 CPUs. For the most difficult case, the optimization at $R = 2.25$ Å, nine iterations were required for convergence.

To extrapolate to infinite bond dimension, we followed the standard procedure[15] and did a linear extrapolation of the energy as function of discarded weight. For the linear fit we use data points obtained from a backward propagation, starting with the largest bond dimension and successively reoptimizing the matrix product state at smaller bond dimensions. The energy is a linear function of discarded weight in the limit of small discarded weight. However at the largest bond dimension, the wavefunctions are imperfectly optimized (as they do not have information from states with much larger bond dimension), while at the smallest bond dimension, the discarded weight may be too large to be in the linear regime.

[a)]Electronic mail: garnetc [a t] caltech . edu
[b)]Electronic mail: larsson22_cr2 [a t] larsson-research. de

Consequently, we discard the data of the largest bond dimensions and smallest bond dimensions if it significantly worsens $R^2$. To account for outliers, we used a robust least-squares fit with a Huber loss function.[16] The raw and extrapolated DMRG energies, together with the bond dimensions used for the optimizations and for the fits are shown in Table S2.

It should be emphasized that the SHCI and DMRG extrapolations are ultimately uncontrolled procedures; the method of extrapolation is not unique and estimating the error of the extrapolation is difficult, and this is the importance of having two different estimates. However, the estimated extrapolated energies are in good agreement with each other. Note also that the assignments of vibrational quantum numbers do not change for reasonable variants of the extrapolation procedure.

### B. Basis set correction

To account for the basis-set correction, we use the second order uncontracted multireference retaining the excitation degree perturbation theory (MRREPT) wavefunction, approximated by a matrix product state (MPS). (Although this is strictly a matrix product state perturbation theory,[3] this approximation was termed matrix product state linearized coupled cluster theory (MPS-LCC) in the literature, because of a connection to coupled cluster theory in the limit of a single reference theory.[4] However, to avoid confusion with other methods also referred to as multireference linearized coupled cluster,[17,18] we refer to the method as MPS-REPT2 in the following). We computed the MPS-REPT2 energies using BLOCK2.[5,10] We used the cc-pV$N$Z-DK basis set, which includes up to $i$-type functions for $N = 5$.[19] While the basis set superposition error (BSSE) can be very large in $Cr_2$ for small bases,[20,21] we did not employ any approximate BSSE correction because we include up to quintuple zeta bases and extrapolate to the basis set limit, where the BSSE is zero, by definition. BSSE corrections have been omitted in other studies as well.[12,22,23]

The multireference simulations were based on a complete active space self-consistent field (CASSCF) reference with a standard valence CAS(12,12) consisting of 12 electrons and 12 orbitals (3d and 4s), which can be described by 28784 spin-adapted configuration state functions. We optimized the CASSCF wavefunction using the PySCF program package.[8,9] The MPS-REPT2 computations were based on the aforementioned CAS(12,12) and, in addition, correlated the eight 3s and 3p orbitals (internal space) with up to two-fold excitations into the active and external spaces. The MPS used to approximate the MRREPT2 wavefunction included $U(1)$ symmetry-adaptation for $N_{\rm el}$ and $S_z$ and two large sites at either end to describe the internal and external space.[5] We used a bond dimension of up to $D = 16,000$, without further extrapolation of the energy. The PECs were generated from the binding energies as obtained by subtracting twice the atomic energy (the MRREPT theory is fully size consistent). For the largest basis, one MPS-REPT2 iteration (sweep) at $D = 16,000$ took around 7 hours on one node with 56 Intel Xeon 8276 CPUs. Starting from a good guess, for example from a previously computed bond distance, fewer than six iterations are typically required to reach convergence.

*a. MPS-REPT2 PEC* For comparison, the raw MPS-REPT2 PECs for various basis sets are shown in Figure S1. The CBS limit is obtained as shown in the next Section, S1 C. Note that the convergence with the basis set size is not monotonic and the cc-pVDZ-DK binding energies are lower than the cc-pVTZ-DK energies. This non-monotonic basis set convergence has often been observed for $Cr_2$.[5,12] Due to error cancellation, the cc-pVDZ-DK PEC qualitatively agrees with the experimental curve but predicts a too large equilibrium distance. The TZ PEC exhibits a noticable double minimum whereas the CBS PEC does not. This is related to the unusually difficult basis set convergence, and has also been observed elsewhere, e.g., in Refs. 20,23. In contrast to other multi-reference perturbation theories based on a CAS(12,12) reference, the raw MPS-REPT2 CBS curve shows surprisingly good agreement with the experimental Casey-Leopold curve as well as the rederived experimental curve from this work, with a maximal error 0.13 eV, indicating its usefulness as basis set and dynamical correlation correction.

### C. Basis set extrapolation

We calculated $\Delta E_{\rm CBS}$(MPS-REPT2) by fitting the binding energies to

$$\Delta E(\mathcal{N}) = \Delta E_{\rm CBS} + A(\mathcal{N} + 1/2)^{-3}, \qquad \text{(S2)}$$

where $\mathcal{N}$ is the cardinal number of the basis set. We use triple, quadruple, and quintuple zeta bases for the fit.

### D. Error estimates

Equation S1 contains error contributions from three main sources: (1) The PDZ energy for the cc-pVDZ-DK basis set, $\Delta E_{\rm PDZ}$, (2) the basis set extrapolation energy, $\Delta E_{CBS}$(MPS-REPT2), and (3) the error from the approximate nature of the MPS-REPT2 method. Additional errors that we neglect here come from, e.g., the approximate nature of the relativistic two-component Hamiltonian (which is, however, mostly addressed by the basis set extrapolation because it is exact in the complete basis set limit), non-Born-Oppenheimer corrections, and the spline interpolation error (because the MPS-REPT2 energies were computed at different points but on a denser grid than the SHCI energies). We calculate the total error assuming that the individual contributions are independent (see below).

TABLE S2. DMRG energies at the cc-pVDZ-DK level. $D_{\mathrm{max}}$ is the maximal bond dimension used for the optimization. $D^{\mathrm{fit}}_{\mathrm{min}}$ ($D^{\mathrm{fit}}_{\mathrm{max}}$) are the minimal (maximal) bond dimensions used for the fit to extrapolate the energy to infinite bond dimension, $E(\infty)$. The energies are shifted by 2099 $\mathrm{E_H}$. $\mathrm{R}^2$ is the coefficient of determination of the linear fit.

| $R$ /Å | $D_{\mathrm{max}}$ | $D^{\mathrm{fit}}_{\mathrm{min}}$ | $D^{\mathrm{fit}}_{\mathrm{max}}$ | $E(D_{\mathrm{max}})$ /$\mathrm{E_H}$ | $E(\infty)$ /$\mathrm{E_H}$ | $E(D_{\mathrm{max}})$ - $E(\infty)$ /$\mathrm{mE_H}$ | $\mathrm{R}^2$ |
|---|---|---|---|---|---|---|---|
| 1.50 | 18 000 | 6000 | 17 000 | −0.8852 | −0.8929 | 8 | 0.998 |
| 1.55 | 18 000 | 8000 | 18 000 | −0.9001 | −0.9084 | 8 | 0.998 |
| 1.60 | 18 000 | 8000 | 18 000 | −0.9083 | −0.9177 | 9 | 0.998 |
| 1.68 | 25 000 | 8000 | 22 000 | −0.9150 | −0.9227 | 8 | 0.997 |
| 1.80 | 25 000 | 10 000 | 24 000 | −0.9134 | −0.9221 | 9 | 0.995 |
| 2.00 | 25 000 | 10 000 | 22 000 | −0.9074 | −0.9183 | 11 | 0.992 |
| 2.25 | 28 000 | 14 000 | 27 000 | −0.9063 | −0.9131 | 7 | 0.998 |
| 2.50 | 18 000 | 8000 | 17 000 | −0.9014 | −0.9096 | 8 | 0.997 |
| 2.75 | 18 000 | 6000 | 17 000 | −0.8969 | −0.9047 | 8 | 0.995 |
| 3.00 | 18 000 | 6000 | 16 000 | −0.8906 | −0.8979 | 8 | 0.995 |
| 3.25 | 18 000 | 6000 | 16 000 | −0.8838 | −0.8911 | 8 | 0.991 |

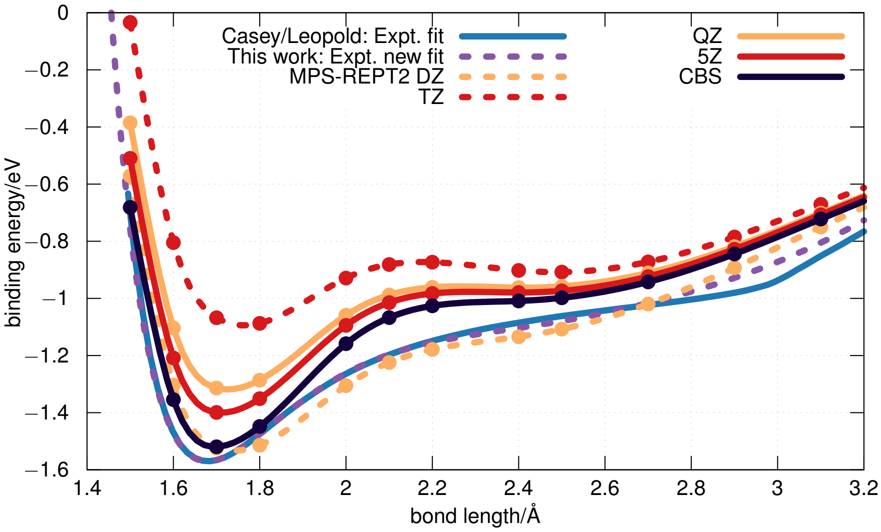


FIG. S1. Potential energy curves of the chromium dimer. The blue curve show the experimental result from Casey and Leopold.[24] The dotted purple curve is our new fit based on the reassigned experimental data. The other curves show MPS-REPT2 results in different bases and for the basis set limit (CBS).

We now discuss how we calculate the individual error estimates. (1) We estimated the error bar of the PDZ energy to be half the absolute difference of the DMRG and the SHCI energies, which is identical to the standard deviation of the mean of two separate measurements.[25] Note that both SHCI and DMRG are methods that can systematically approximate and extrapolate to the exact energy but work in a very different way, thus the estimates of the energy are roughly independent. (2) We compute the basis set extrapolation error from the standard deviation $\sigma_{\mathrm{CBS}}$ obtained by the least-squares fit of Eq. S2. A more conservative alternative is to define the error bar as the difference between the extrapolation with and without the largest basis set. This gives an error that is slightly ($\sim 0.002\,\mathrm{eV}$) larger but which follows the same trend as that computed from the fit. (3) We conservatively estimated the error bar of the MPS-REPT2-based correction by taking half the absolute difference between the values of the UCCSD(T) correction from Li et al.[12] and that from MPS-REPT2. Due to the poor quality of the UCCSD(T) PECs we believe that this overestimates the error bar. An alternative would be to estimate the error as some fraction, e.g. $\sim 20\,\%$ of the correction. For $R \to \infty$, the binding energy approaches zero, which also holds for this definition of the error. This type of error estimate leads to errors that are a factor of $\sim 2$ smaller than the UCCSD(T)-estimated errors. Another alternative would be to compare to the MPS-REPT3-based third order perturbative correction, which we computed as well. For $R \geq 2\,$Å, the error based on $20\,\%$ of the correction and the MPS-REPT3-based error are roughly similar and for $R < 2\,$Å the MPS-REPT3-based error gets too large, larger than even the UCCSD(T)-based error. The problematic behavior of third order perturbation theory at $R < 2\,$Å has also been seen in n-Electron Valence State Perturbation-Theory (NEVPT3).[26]

Assuming that the individual errors are indepen-

dent, the total error is then given as[25]

$$\epsilon = \sqrt{\epsilon_{\mathrm{PDZ}}^2 + \epsilon_{\mathrm{CBS}}^2 + \epsilon_{\mathrm{REPT}}^2}, \tag{S3}$$

with the individual error contributions as defined above,

$$\epsilon_{\mathrm{PDZ}} = |\Delta E(\mathrm{SHCI}) - \Delta E(\mathrm{DMRG})|/2, \tag{S4}$$
$$\epsilon_{\mathrm{CBS}} = \sigma_{\mathrm{CBS}}, \tag{S5}$$
$$\epsilon_{\mathrm{REPT}} = |\Delta E(\text{MPS-REPT2}) - \Delta E[\mathrm{UCCSD(T)}]|/2. \tag{S6}$$

## S2. VIBRATIONAL SPECTRUM

We simulated the vibrational spectrum of $^{52}\mathrm{Cr}^{52}\mathrm{Cr}$ and $^{50}\mathrm{Cr}^{52}\mathrm{Cr}$ by solving the $J = 0$ vibrational Schrödinger equation using the sine discrete variable representation (DVR)[27] with 1000 grid points placed between $\sim 1.40$ Å and $\sim 3.45$ Å. We represented the potential by cubic spline interpolation. As atomic masses we used 51.9405115 u for $^{52}$Cr and 49.9460495 u for $^{50}$Cr.[28]

## S3. POTENTIAL ENERGY CURVE FIT

To obtain an analytical PEC based on the available vibrational data, we solved the inverse Schrödinger equation using 180 DVR grid points and we expressed the PEC using the expanded Morse oscillator (EMO) form:[29–33]

$$V_{\mathrm{EMO}}(R) = D\{1 - \exp[-\beta(R)(R - R_e)]\}^2, \tag{S7}$$
$$\beta(R) = \sum_{i=0}^{N_p} a_i[(R^q - r_r^q)/(R^q + r_r^q)]^i. \tag{S8}$$

For the fit we used a polynomial order of $N_p = 4$ for the evaluation of $\beta(R)$ and chose $q = 5$. We kept $R_e$ fixed at the experimental value of 1.6788 Å. All other values, including $r_r$, were optimized.

Following Casey and Leopold, we included in the fit the first nine vibrational levels and the 20 vibrational levels starting at 4880 cm$^{-1}$.[24] Likewise, we did not include the two levels at 4290 cm$^{-1}$ and 4570 cm$^{-1}$ in the fit, as those are difficult to assign and Casey and Leopold suggested that the transitions may not stem from the $^1\Sigma_g^+$ $\mathrm{Cr}_2$ ground state. We solved the inverse Schrödinger equation using least-squares fitting with the Jacobian obtained by automated differentiation using the JAX library.[34] We note that many different potential energy curves (different fit results) lead to an excellent agreement with the experimental levels. There is hence a large uncertainty in the derived experimental PEC. Here we chose a fit that both has an excellent agreement with the experimental levels and that is sufficiently smooth. Including the two 4290/4570 cm$^{-1}$ levels in the fit resulted in a PEC with small wiggles in the region of 2.2–3.0 Å but did not lead to changes in the overall shape. The final values of the EMO potential are listed in Table S3.

TABLE S3. Parameter values of the expanded Morse oscillator fit, Equation S8. The cluster of vibrational levels at 4880 cm$^{-1}$ are assigned to $v = 23 - 42$.

| Parameter | value |
|---|---|
| $D$/cm$^{-1}$ | 12 959.4 |
| $r_r$/Å | 2.794 295 |
| $a_0$/Å$^{-1}$ | 0.836 801 |
| $a_1$/Å$^{-2}$ | −0.270 609 |
| $a_2$/Å$^{-3}$ | 0.787 853 |
| $a_3$/Å$^{-4}$ | −0.110 491 |
| $a_4$/Å$^{-5}$ | 1.684 039 |

## S4. VIBRATIONAL ASSIGNMENT AND PEC EVALUATION

The experimental vibrational levels are compared with our new EMO fit and our simulated PEC, which is based on our composite method, in Table S4. Casey and Leopold's original assignment[24] of the cluster starting at 4880 cm$^{-1}$ was obtained by comparing the experimental vibrational energies to those obtained from a slightly modified Rydberg-Klein-Rees potential for various assignments for the vibrational levels. Casey and Leopold stated that $v = 22$–41 was the lowest vibrational numbering that leads to agreement between the observed and the vibrational levels obtained via a PEC generated from a modified Rydberg-Klein-Rees (RKR) method.[35–38] The assignment of $v = 24$–43 gave a good agreement also with the two levels at 4290 cm$^{-1}$ and 4570 cm$^{-1}$, that were assigned to $v = 18$ and $v = 21$, respectively, based on the obtained RKR potential. However, they stated that these transitions may not stem from the $^1\Sigma_g^+$ $\mathrm{Cr}_2$ ground state. They did a further check by comparing the isotope shift of seven levels between 5240 cm$^{-1}$ and 6000 cm$^{-1}$. The observed isotope shift was $24 \pm 8$ cm$^{-1}$ whereas that of the modified RKR potential is 36 cm$^{-1}$. Only when assigning the higher levels as $v = 20$–39 could they obtain a potential with an isotope shift within experimental uncertainty (31 cm$^{-1}$), but the resulting potential had a large error for the $v = 9$ level. Similar to that of the modified RKR potential, our simulated composite curve also results in an average isotope shift of 36 cm$^{-1}$ in this region. The newly fitted EMO potential results in a slightly lower average isotope shift of 35 cm$^{-1}$.

TABLE S4: Measured and simulated vibrational energy levels. Units are in $cm^{-1}$. The experimental data for $v = 1$ is from Ref. 39. All other exp. data is from Ref. 24. ZPE stands for zero point energy, relative to a potential with minimum energy of 0. The values for $v > 0$ are relative to the ground state energy. $\tilde{\nu}^o$ ($\tilde{\nu}^n$) are the vibrational levels for the old (new) assignment for the states starting at 4880 $cm^{-1}$ and for the state at 4290 $cm^{-1}$. The assignment of the exp. levels in parentheses is not fully clear and these levels may not belong to the $Cr_2$ ground state.[24] $\tilde{\nu}_{\mathrm{EMO}}$ are the levels for the extended Morse oscillator fit based on the new assignment, and $\tilde{\nu}_{\mathrm{theory}}$ are the levels from our composite theory. The difference between theory and experiment is an order of magnitude smaller for the new assignment than for the old assignment and is comparable to the experimental uncertainty.

| $v$ | $\tilde{\nu}^o_{\mathrm{exp}}$ | $\tilde{\nu}^n_{\mathrm{exp}}$ | $\tilde{\nu}_{\mathrm{EMO}}$ | $\tilde{\nu}^n_{\mathrm{exp}} - \tilde{\nu}_{\mathrm{EMO}}$ | $\tilde{\nu}_{\mathrm{theory}}$ | $\tilde{\nu}^o_{\mathrm{exp}} - \tilde{\nu}_{\mathrm{theory}}$ | $\tilde{\nu}^n_{\mathrm{exp}} - \tilde{\nu}_{\mathrm{theory}}$ |
|---|---|---|---|---|---|---|---|
| ZPE | | | 236.15 | | 242.77 | | |
| 1 | 452.34±0.02 | same | 452.34 | 0 | 467.84 | -16 | |
| 2 | 875±10 | same | 877.6 | -3 | 900.7 | -26 | |
| 3 | 1280±10 | same | 1275.2 | 5 | 1293.6 | -14 | |
| 4 | 1645±10 | same | 1644.7 | 0 | 1652.1 | -7 | |
| 5 | 1985±15 | same | 1985.4 | -0 | 1980.1 | 5 | |
| 6 | 2300±15 | same | 2296.5 | 3 | 2278.7 | 21 | |
| 7 | 2580±20 | same | 2577.1 | 3 | 2548.0 | 32 | |
| 8 | 2830±20 | same | 2826.1 | 4 | 2790.1 | 40 | |
| 9 | 3040±20 | same | 3042.9 | -3 | 3005.0 | 35 | |
| 10 | | | 3228.2 | | 3193.7 | | |
| 11 | | | 3386.3 | | 3358.1 | | |
| 12 | | | 3525.3 | | 3502.2 | | |
| 13 | | | 3654.1 | | 3631.6 | | |
| 14 | | | 3778.2 | | 3752.9 | | |
| 15 | | | 3900.3 | | 3871.0 | | |
| 16 | | | 4021.4 | | 3988.5 | | |
| 17 | | | 4142.2 | | 4106.5 | | |
| 18 | (4290±20) | | 4262.9 | (27) | 4225.6 | (64) | |
| 19 | | (4290±20) | 4383.8 | (-94) | 4346.2 | | (-56) |
| 20 | | | 4504.9 | | 4468.5 | | |
| 21 | (4570±20) | (same) | 4626.3 | (-56) | 4592.4 | (-22) | |
| 22 | | | 4748.2 | | 4717.8 | | |
| 23 | | 4880±20 | 4870.5 | 9 | 4844.4 | | 36 |
| 24 | 4880±20 | 5000±15 | 4993.4 | 7 | 4972.1 | -92 | 28 |
| 25 | 5000±15 | 5115±15 | 5117.0 | -2 | 5100.8 | -101 | 14 |
| 26 | 5115±15 | 5240±15 | 5241.2 | -1 | 5230.3 | -115 | 10 |
| 27 | 5240±15 | 5360±15 | 5366.1 | -6 | 5360.4 | -120 | -0 |
| 28 | 5360±15 | 5490±15 | 5491.8 | -2 | 5491.1 | -131 | -1 |
| 29 | 5490±15 | 5615±15 | 5618.3 | -3 | 5622.2 | -132 | -7 |
| 30 | 5615±15 | 5745±15 | 5745.5 | -0 | 5753.5 | -138 | -8 |
| 31 | 5745±15 | 5870±15 | 5873.5 | -4 | 5884.9 | -140 | -15 |
| 32 | 5870±15 | 6000±15 | 6002.3 | -2 | 6016.6 | -147 | -17 |
| 33 | 6000±15 | 6135±15 | 6132.0 | 3 | 6148.6 | -149 | -14 |
| 34 | 6135±15 | 6265±15 | 6262.3 | 3 | 6280.6 | -146 | -16 |
| 35 | 6265±15 | 6400±15 | 6393.5 | 7 | 6412.3 | -147 | -12 |
| 36 | 6400±15 | 6530±15 | 6525.3 | 5 | 6543.8 | -144 | -14 |
| 37 | 6530±15 | 6660±20 | 6657.9 | 2 | 6675.1 | -145 | -15 |
| 38 | 6660±20 | 6790±20 | 6791.1 | -1 | 6806.0 | -146 | -16 |
| 39 | 6790±20 | 6920±20 | 6925.0 | -5 | 6936.2 | -146 | -16 |
| 40 | 6920±20 | 7060±20 | 7059.4 | 1 | 7066.0 | -146 | -6 |
| 41 | 7060±20 | 7190±20 | 7194.5 | -4 | 7195.1 | -135 | -5 |
| 42 | 7190±20 | 7320±20 | 7330.0 | -10 | 7323.3 | -133 | -3 |
| 43 | 7320±20 | | 7466.1 | | 7450.8 | -131 | |

## S5. EXPERIMENTAL UNCERTAINTY OF THE POTENTIAL ENERGY CURVE

To estimate the overall uncertainty in the potential energy curve, as shown by the blue-shaded area in Figure 2 (a), we tried out various assignments and sampled different fits that match these assignments equally well. Similar to Casey and Leopold, we found that the quantum number of the vibrational energies above 4880 $cm^{-1}$ can be assigned by starting at one of the following values $v_{\mathrm{prog}} = 21, 22, 23, 24$, and $v_{\mathrm{prog}} = 25$. For all these five assignments PECs can be found with matching frequencies. Figure S2 shows examples of possible curves with different $v_{\mathrm{prog}}$ that all lead to excellent agreement with the experimental vibrational energy levels (max. error of 14 $cm^{-1}$, well within the average experimental uncertainty). Note that many other fits are possible, as indicated by the difference between the $v_{\mathrm{prog}} = 23$ curve (blue line) and our final new fit (dashed purple line), which also

is based on $v_{\mathrm{prog}} = 23$ but overall has a smaller error. We note that we did not include the experimental isotope shift of some of the vibrational levels obtained from Casey and Leopold as an additional measure of quality in this procedure, because the isotope shift itself is only given with large error ($24 \pm 8\,\mathrm{cm}^{-1}$) and the final PEC obtained by Casey and Leopold also disagrees with this (average shift of $36\,\mathrm{cm}^{-1}$). For these five assignments and for the final assignment from Casey and Leopold that includes the two $4290/4570\,\mathrm{cm}^{-1}$ levels we drew $7 \cdot 10^5$ random samples of the experimentally observed frequencies within their experimental uncertainty. Based on these sampled frequencies, we used the RKR method to obtain a first guess of the experimental PEC. We then refined that guess using the EMO potential. Finally, from all these $6 \cdot 7 \cdot 10^5 \approx 4 \cdot 10^6$ PECs we selected those that match all experimentally observed frequencies within their experimental uncertainty. At each bond length, we then used the extrema of these set of PECs as an estimate of the experimental uncertainty in the potential energy curve shown as the blue-shaded area in Figure 2 (a).

TABLE S5: Measured and simulated spectroscopic constants for the $X\,^1\Sigma_g^+$ state of $Cr_2$. The experimental values of $D_e$ assume a vibrational zero-point energy of 0.029 eV. The composite method used in this work gave a zero-point energy of 0.030 eV. If the original literature did not contain all constants, we computed the constants and show them in square brackets. For $\omega_e$, we use a fit to a second-order Dunham expansion of the lowest 9 vibrational levels. For comparison, we show the so-obtained $\omega_e$ also if the original data is available. Note that the original values in Ref. 22 use a different PEC than the recomputed ones, because the used PEC is not displayed. The data is used for Figure 3 in the main text. Note that the experimental value of $D_e$ ($D_0$) from Ref. 40 may be too large, as the authors assumed that the $^2\Sigma_g^+$ state is the ground state of $Cr_2{}^+$. Recent experiments indicate that the configuration of the ground state of $Cr_2{}^+$ is $^{12}\Sigma_u^+$.[41] Similarly, the value of $D_e$ ($D_0$) from Ref. 42 may be too small, as the analysis did not take into account the contributions of electronically excited states.

| method | $r_e$/Å | $D_e$/eV | $\omega_e$/cm$^{-1}$ | $\Delta G_{1/2}$/cm$^{-1}$ |
|---|---|---|---|---|
| | | this work | | |
| composite method | 1.685 | 1.58±0.02 | 495 | 468 |
| MPS-REPT2 | 1.700 | 1.52 | 477 | 458 |
| | | other work | | |
| semiempirical[43] | 2.5 | 1.05 | | |
| extended Hückel[44] | 1.7 | 1.6 | | |
| SCF-X$\alpha$-SW[44] | 1.9 | | | |
| GVB-vdW[45] | 3.0±0.6 | 0.3±0.05 | 110 [106] | 108 |
| MGVB[46] | 1.61 | 1.86 | [600] | [547] |
| CCSD(T)[47] | 1.604 | | 766 | |
| CCSD(T)[48] | 1.59 | 0.38 | | |
| UCCSD(T)[48] | 2.54 | 0.89 | [174] | [174] |
| UBLYP[48] | 1.7 | 1.99 | [415] | [400] |
| CASPT2[49] | 1.71 | 1.583 | 625 [591] | [574] |
| CASPT2[50] | 1.686 | 1.538 | 550 [544] | 535 |
| SP-B3P86[51] | 1.59 | 1.38 | [502] | [427] |
| MRACPF[52] | 1.73 | 1.12 | 318 [358] | [324] |
| MRACPF[53] | 1.72 | 1.09 | 339 [148] | [235] |
| sc-NEVPT2[54] | 1.662 | 1.493 | 575 [560] | [552] |
| CASPT2[55] | 1.662 | 1.618 | 413 [445] | [410] |
| MRCIPT2+Q[56] | 1.756 | 1.18 | 332 [344] | [311] |
| MRCI+Q[56] | 1.666 | 1.07 | 512 | |
| MRAQCC[20] | 1.685 | 1.355 | 459 [423] | 431 |
| RASPT2[57] | 1.687 | 1.6 | | 516 |
| MPS-CASPT2[22] | 1.681 | 1.61 | 480 [516] | [489] |
| SplitGAS[58] | 1.671 | 1.56 | 484.8 | |
| DMRG-ec-MRCI+Q[59] | 1.71 | 1.62 | 477 [496] | [482] |
| iSUPT2[60] | [1.59] | [1.35] | [681] | [456] |
| FP-AFQMC[61] | 1.65±0.02 | 1.63±0.05 | 552±93 [541] | [478] |
| GASPT2[62] | 1.67 | 1.42 | | |
| RASPT2[21] | 1.666 | 1.89 | 489 [468] | [464] |
| MPS-NEVPT2[23] | 1.656 | 1.43 | 470 [435] | [422] |
| SHCI+UCCSD(T)[12] | [1.683] | [1.551] | [448] | [428] |
| | | experiment | | |
| | 1.71[63] | 1.56±0.3[64] | | |
| | 1.6788[39] | 1.472±0.06[42] | 480.6±0.5[24] | 455±10[24] |
| | | 1.45±0.1[65] | 470[39] | 452.34±0.02[39] |
| | | 1.56±0.06[40] | | |

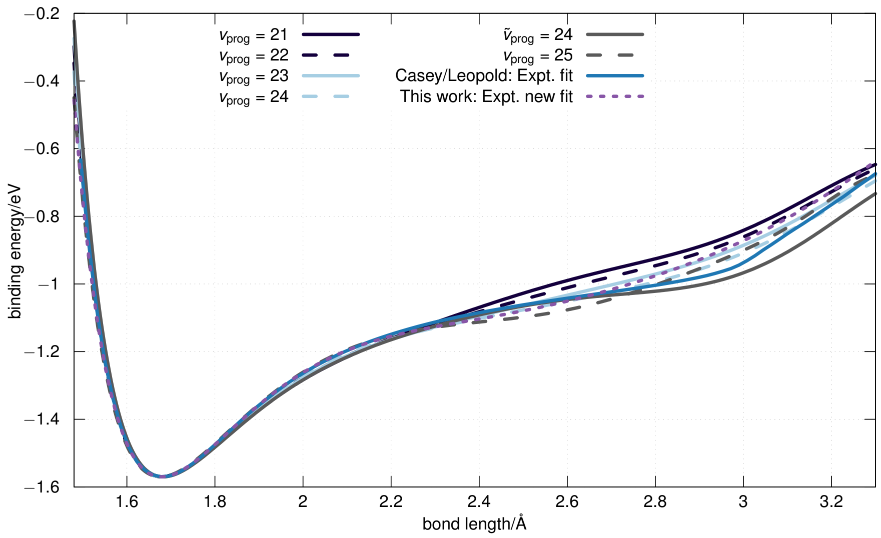


FIG. S2. Examples of various expanded Morse oscillator PEC fits to the experimental vibrational data. $v_{\mathrm{prog}}$ denotes the start of the cluster of 20 vibrational levels. $\tilde{v}_{\mathrm{prog}}$ denotes that the additional vibrational levels at $4290\,\mathrm{cm}^{-1}$ and $4570\,\mathrm{cm}^{-1}$ are included in the fit as $v = 18$ and $v = 21$, respectively.

## S6. REFERENCE LIST FOR FIGURE 1

- 1981 Ref. 45
- 1983 Ref. 66
- 1985 Ref. 46
- 1994a Ref. 49
- 1994b/1994c Ref. 48
- 1995a Ref. 51
- 1995b Ref. 50
- 1996 Ref. 52
- 1999 Ref. 53
- 2001 Ref. 67
- 2003 Ref. 55
- 2004 Ref. 56
- 2009 Ref. 20
- 2011 Ref. 22
- 2015 Ref. 61
- 2016a Ref. 21
- 2016b Ref. 23
- 2018 Ref. 59
- 2019 Ref. 60
- 2020 Ref. 12


[1] Dunning, T. H. Gaussian basis sets for use in correlated molecular calculations. I. The atoms boron through neon and hydrogen. *J. Chem. Phys.* **1989**, *90*, 1007–1023.

[2] Fink, R. F. The multi-reference retaining the excitation degree perturbation theory: A size-consistent, unitary invariant, and rapidly convergent wavefunction based ab initio approach. *Chem. Phys.* **2009**, *356*, 39–46.

[3] Sharma, S.; Chan, G. K.-L. Communication: A flexible multireference perturbation theory by minimizing the Hylleraas functional with matrix product states. *J. Chem. Phys.* **2014**, *141*, 111101.

[4] Sharma, S.; Alavi, A. Multireference linearized coupled cluster theory for strongly correlated systems using matrix product states. *J. Chem. Phys.* **2015**, *143*, 102815.

[5] Larsson, H. R.; Zhai, H.; Gunst, K.; Chan, G. K.-L. Matrix Product States with Large Sites. *J. Chem. Theory Comput.* **2022**, *18*, 749–762.

[6] Peng, D.; Reiher, M. Exact Decoupling of the Relativistic Fock Operator. *Theor. Chem. Acc.* **2012**, *131*, 1081.

[7] Kutzelnigg, W.; Liu, W. Quasirelativistic Theory Equivalent to Fully Relativistic Theory. *J. Chem. Phys.* **2005**, *123*, 241102.

[8] Sun, Q.; Berkelbach, T. C.; Blunt, N. S.; Booth, G. H.; Guo, S.; Li, Z.; Liu, J.; McClain, J. D.; Sayfutyarova, E. R.; Sharma, S.; Wouters, S.; Chan, G. K. PySCF: the Python-based simulations of chemistry framework. *WIREs Comput Mol Sci* **2017**, *8*, e1340.

[9] Sun, Q. et al. Recent developments in the PySCF program package. *J. Chem. Phys.* **2020**, *153*, 024109.

[10] Zhai, H.; Chan, G. K.-L. Low Communication High Performance Ab Initio Density Matrix Renormalization Group Algorithms. *J. Chem. Phys.* **2021**, *154*, 224116.

[11] Li, J.; Otten, M.; Holmes, A. A.; Sharma, S.; Umrigar, C. J. Fast Semistochastic Heat-Bath Configuration Interaction. *J. Chem. Phys.* **2018**, *149*, 214110.

[12] Li, J.; Yao, Y.; Holmes, A. A.; Otten, M.; Sun, Q.; Sharma, S.; Umrigar, C. J. Accurate many-body electronic structure near the basis set limit: Application to the chromium dimer. *Phys. Rev. Research* **2020**, *2*, 012015.

[13]https://github.com/QMC-Cornell/shci.
[14]Guo, S.; Li, Z.; Chan, G. K.-L. A Perturbative Density Matrix Renormalization Group Algorithm for Large Active Spaces. *J. Chem. Theory Comput.* **2018**, *14*, 4063–4071.
[15]Olivares-Amaya, R.; Hu, W.; Nakatani, N.; Sharma, S.; Yang, J.; Chan, G. K.-L. The *Ab-Initio* Density Matrix Renormalization Group in Practice. *J. Chem. Phys.* **2015**, *142*, 034102.
[16]Boyd, S. *Convex optimization*, 1st ed.; Cambridge University Press: Cambridge, UK, 2004.
[17]Laidig, W. D.; Saxe, P.; Bartlett, R. J. The description of $N_2$ and $F_2$ potential energy surfaces using multireference coupled cluster theory. *J. Chem. Phys.* **1987**, *86*, 887–907.
[18]Black, J. A.; Köhn, A. Linear and quadratic internally contracted multireference coupled-cluster approximations. *J. Chem. Phys.* **2019**, *150*, 194107.
[19]Balabanov, N. B.; Peterson, K. A. Systematically Convergent Basis Sets for Transition Metals. I. All-Electron Correlation Consistent Basis Sets for the 3d Elements Sc–Zn. *J. Chem. Phys.* **2005**, *123*, 064107.
[20]Müller, T. Large-Scale Parallel Uncontracted Multireference-Averaged Quadratic Coupled Cluster: The Ground State of the Chromium Dimer Revisited. *J. Phys. Chem. A* **2009**, *113*, 12729–12740.
[21]Vancoillie, S.; Malmqvist, P. A.; Veryazov, V. Potential Energy Surface of the Chromium Dimer Re-re-revisited with Multiconfigurational Perturbation Theory. *J Chem Theory Comput* **2016**, *12*, 1647–1655.
[22]Kurashige, Y.; Yanai, T. Second-order perturbation theory with a density matrix renormalization group self-consistent field reference function. *J. Chem. Phys.* **2011**, *135*, 094104.
[23]Guo, S.; Watson, M. A.; Hu, W.; Sun, Q.; Chan, G. K.-L. *N* -Electron Valence State Perturbation Theory Based on a Density Matrix Renormalization Group Reference Function, with Applications to the Chromium Dimer and a Trimer Model of Poly(*p*-Phenylenevinylene). *J. Chem. Theory Comput.* **2016**, *12*, 1583–1591.
[24]Casey, S. M.; Leopold, D. G. Negative Ion Photoelectron Spectroscopy of Chromium Dimer. *J. Phys. Chem.* **1993**, *97*, 816–830.
[25]Taylor, J. R. *An Introduction to Error Analysis: The Study of Uncertainties in Physical Measurements*, 2nd ed.; University Science Books, 1997; p 327.
[26]Angeli, C.; Bories, B.; Cavallini, A.; Cimiraglia, R. Third-Order Multireference Perturbation Theory: The n-Electron Valence State Perturbation-Theory Approach. *J. Chem. Phys.* **2006**, *124*, 054108.
[27]Colbert, D. T.; Miller, W. H. A Novel Discrete Variable Representation for Quantum Mechanical Reactive Scattering via the *S* -matrix Kohn Method. *J. Chem. Phys.* **1992**, *96*, 1982–1991.
[28]de Laeter, J. R.; Böhlke, J. K.; Bièvre, P. D.; Hidaka, H.; Peiser, H. S.; Rosman, K. J. R.; Taylor, P. D. P. Atomic weights of the elements. Review 2000 (IUPAC Technical Report). *Pure Appl. Chem.* **2003**, *75*, 683–800.
[29]Lee, E. G.; Seto, J. Y.; Hirao, T.; Bernath, P. F.; Le Roy, R. J. FTIR Emission Spectra, Molecular Constants, and Potential Curve of Ground State GeO. *J. Mol. Spectrosc.* **1999**, *194*, 197–202.
[30]Hedderich, H. G.; Dulick, M.; Bernath, P. F. High Resolution Emission Spectroscopy of AlCl at 20 $\mu$. *J. Chem. Phys.* **1998**, *99*, 8363.
[31]Coxon, J. A.; Hajigeorgiou, P. G. Isotopic Dependence of Born-Oppenheimer Breakdown Effects in Diatomic Hydrides: The $B^1\Sigma^+$ and $X^1\Sigma^+$ States of HCl and DCl. *J. Mol. Spectrosc.* **1990**, *139*, 84–106.
[32]Le Roy, R. J. dPotFit: A Computer Program to Fit Diatomic Molecule Spectral Data to Potential Energy Functions. *J. Quant. Spectrosc. Radiat. Transf.* **2017**, *186*, 179–196.
[33]Šurkus, A. A.; Rakauskas, R. J.; Bolotin, A. B. The Generalized Potential Energy Function for Diatomic Molecules. *Chem. Phys. Lett.* **1984**, *105*, 291–294.
[34]Bradbury, J.; Frostig, R.; Hawkins, P.; Johnson, M. J.; Leary, C.; Maclaurin, D.; Necula, G.; Paszke, A.; VanderPlas, J.; Wanderman-Milne, S.; Zhang, Q. JAX: composable transformations of Python+NumPy programs. 2021; http://github.com/google/jax.
[35]Rees, A. L. G. The Calculation of Potential-Energy Curves from Band-Spectroscopic Data. *Proc. Phys. Soc.* **1947**, *59*, 998–1008.
[36]Rydberg, R. Graphische Darstellung einiger bandenspektroskopischer Ergebnisse. *Z. Physik* **1932**, *73*, 376–385.
[37]Klein, O. Zur Berechnung von Potentialkurven für zweiatomige Moleküle mit Hilfe von Spektraltermen. *Z. Physik* **1932**, *76*, 226–235.
[38]Le Roy, R. J. RKR1: A Computer Program Implementing the First-Order RKR Method for Determining Diatomic Molecule Potential Energy Functions. *J. Quant. Spectrosc. Radiat. Transf.* **2017**, *186*, 158–166.
[39]Bondybey, V. E.; English, J. H. Electronic Structure and Vibrational Frequency of $Cr_2$. *Chem. Phys. Lett.* **1983**, *94*, 443–447.
[40]Simard, B.; Lebeault-Dorget, M.-A.; Marijnissen, A.; ter Meulen, J. J. Photoionization Spectroscopy of Dichromium and Dimolybdenum: Ionization Potentials and Bond Energies. *J. Chem. Phys.* **1998**, *108*, 9668–9674.
[41]Zamudio-Bayer, V.; Hirsch, K.; Langenberg, A.; Niemeyer, M.; Vogel, M.; Ławicki, A.; Terasaki, A.; Lau, J. T.; von Issendorff, B. Maximum Spin Polarization in Chromium Dimer Cations as Demonstrated by X-ray Magnetic Circular Dichroism Spectroscopy. *Angew. Chem. Int. Ed.* **2015**, *54*, 4498–4501.
[42]Hilpert, K.; Ruthardt, R. Determination of the Dissociation Energy of the Cr $_2$ Molecule. *Ber. Bunsenges. Phys. Chem.* **1987**, *91*, 724–731.
[43]Anderson, A. B. Structures, Binding Energies, and Charge Distributions for Two to Six Atom Ti, Cr, Fe, and Ni Clusters and Their Relationship to Nucleation and Cluster Catalysis. *J. Chem. Phys.* **1976**, *64*, 4046–4055.
[44]Klotzbuecher, W.; Ozin, G. A.; Norman, J. G.; Kolari, H. J. Bimetal Atom Chemistry. 1. Synthesis, Electronic Absorption Spectrum, and Extended Hueckel/Self-Consistent Field-X$\alpha$-Scattered Wave Molecular Orbital Analyses of the Chromium-Molybdenum (CrMo) Molecule: Relevance to Alloy and Bimetallic Cluster Catalysis. *Inorg. Chem.* **1977**, *16*, 2871–2877.
[45]Goodgame, M. M.; Goddard, W. A. The "Sextuple" Bond of Chromium Dimer. *J. Phys. Chem.* **1981**, *85*, 215–217.
[46]Goodgame, M. M.; Goddard, W. A. Modified Generalized Valence-Bond Method: A Simple Correction for the Electron Correlation Missing in Generalized Valence-Bond Wave Functions; Prediction of Double-Well States for $Cr_2$ and $Mo_2$. *Phys. Rev. Lett.* **1985**, *54*, 661–664.
[47]Scuseria, G. E. Analytic Evaluation of Energy Gradients for the Singles and Doubles Coupled Cluster Method Including Perturbative Triple Excitations: Theory and Applications to FOOF and $Cr_2$. *J. Chem. Phys.* **1991**, *94*, 442–447.
[48]Bauschlicher, C. W.; Partridge, H. $Cr_2$ Revisited. *Chem. Phys. Lett.* **1994**, *231*, 277–282.
[49]Andersson, K.; Roos, B. O.; Malmqvist, P. Å.; Widmark, P. O. The $Cr_2$ Potential Energy Curve Studied with Multiconfigurational Second-Order Perturbation Theory. *Chem. Phys. Lett.* **1994**, *230*, 391–397.
[50]Roos, B. O.; Andersson, K. Multiconfigurational Perturbation Theory with Level Shift — the $Cr_2$ Potential Revisited. *Chem. Phys. Lett.* **1995**, *245*, 215–223.
[51]Edgecombe, K. E.; Becke, A. D. $Cr_2$ in Density-Functional Theory: Approximate Spin Projection. *Chem. Phys. Lett.* **1995**, *244*, 427–432.
[52]Stoll, H.; Werner, H. The $Cr_2$ potential curve: a multireference pair functional treatment. *Mol. Phys.* **1996**, *88*, 793–802.
[53]Dachsel, H.; Harrison, R. J.; Dixon, D. A. Multireference Configuration Interaction Calculations on $Cr_2$: Passing the One Billion Limit in MRCI/MRACPF Calculations. *J. Phys. Chem. A* **1999**, *103*, 152–155.

[54]Angeli, C.; Cimiraglia, R.; Evangelisti, S.; Leininger, T.; Malrieu, J.-P. Introduction of N-Electron Valence States for Multireference Perturbation Theory. *J. Chem. Phys.* **2001**, *114*, 10252–10264.

[55]Roos, B. O. The Ground State Potential for the Chromium Dimer Revisited. *Collect. Czech. Chem. Commun.* **2003**, *68*, 265–274.

[56]Celani, P.; Stoll, H.; Werner, H.-J.; Knowles, P. The CIPT2 method: Coupling of multi-reference configuration interaction and multi-reference perturbation theory. Application to the chromium dimer. *Mol. Phys.* **2004**, *102*, 2369–2379.

[57]Ruipérez, F.; Aquilante, F.; Ugalde, J. M.; Infante, I. Complete vs Restricted Active Space Perturbation Theory Calculation of the $Cr_2$ Potential Energy Surface. *J. Chem. Theory Comput.* **2011**, *7*, 1640–1646.

[58]Li Manni, G.; Ma, D.; Aquilante, F.; Olsen, J.; Gagliardi, L. SplitGAS Method for Strong Correlation and the Challenging Case of $Cr_2$. *J. Chem. Theory Comput.* **2013**, *9*, 3375–3384.

[59]Luo, Z.; Ma, Y.; Wang, X.; Ma, H. Externally-Contracted Multireference Configuration Interaction Method Using a DMRG Reference Wave Function. *J. Chem. Theory. Comput.* **2018**, *14*, 4747–4755.

[60]Tsuchimochi, T.; Ten-no, S. L. Second-Order Perturbation Theory with Spin-Symmetry-Projected Hartree–Fock. *J. Chem. Theory Comput.* **2019**, *15*, 6688–6702.

[61]Purwanto, W.; Zhang, S.; Krakauer, H. An Auxiliary-Field Quantum Monte Carlo Study of the Chromium Dimer. *J. Chem. Phys.* **2015**, *142*, 064302.

[62]Ma, D.; Li Manni, G.; Olsen, J.; Gagliardi, L. Second-Order Perturbation Theory for Generalized Active Space Self-Consistent-Field Wave Functions. *J. Chem. Theory Comput.* **2016**, *12*, 3208–3213.

[63]Efremov, Y M,; Samoilova, A N,; Gurvich, L V, Band of $\lambda$=4600 Å produced under a pulsed photolysis of chromium carbonyl. *Opt. Spektrosk.* **1974**, *36*, 654–657.

[64]Kant, A.; Strauss, B. Dissociation Energy of $Cr_2$. *J. Chem. Phys.* **1966**, *45*, 3161–3162.

[65]Su, C.-X.; Hales, D. A.; Armentrout, P. B. The Bond Energies of $Cr_2$ and $Cr_2^+$. *Chem. Phys. Lett.* **1993**, *201*, 199–204.

[66]Walch, P.; Bauschlicher, C. W.; Roos, Björn O.,; Nelin, Constance J., Theoretical evidence for multiple 3D bonding in the $V_2$ and $Cr_2$ molecules. *Chem. Phys. Lett.* **1983**, *103*, 5.

[67]Angeli, C.; Cimiraglia, R.; Malrieu, J.-P. N-Electron Valence State Perturbation Theory: A Fast Implementation of the Strongly Contracted Variant. *Chem. Phys. Lett.* **2001**, *350*, 297–305.
